# Supplementary material for: Improved Metric Distortion for Deterministic Social Choice Rules
Source: arXiv:1905.01401 source file (2019-05-04)
Supplement: Supplementary file 1 [file appendix.tex]

% !TEX root = main.tex
\section{More Discussion on the Experiment}
\label{sec:experiment_extra}
In Section~\ref{sec:experiment}, we use experiment to prove Conjecture~\ref{conjecture} when $|\mathcal{A}| = |\mathcal{C}| + |\mathcal{V}| \leq 14$. Now we are going to discuss about it with more details.

Enumerating all voting profiles for $|\mathcal{A}| \leq 14$ is challenging. For example, when $|\mathcal{C}| = 8$ and $|\mathcal{V}| = 6$, there are $(8!)^6 \approx 4 \times 10^{27}$ different voting profiles. Even after considering the symmetry of voters, there are more than $\frac{(8!)^6}{6!} \approx 6 \times 10^{24}$ different ones.

\textcolor{red}{fill the template}

\IncMargin{1em}
\begin{algorithm}
\SetKwData{Left}{left}\SetKwData{This}{this}\SetKwData{Up}{up}
\SetKwFunction{Union}{Union}\SetKwFunction{FindCompress}{FindCompress}
\SetKwInOut{Input}{input}\SetKwInOut{Output}{output}
\Input{$n = |\mathcal{C}|$, $m = |\mathcal{V}|$, \textcolor{red}{structure}}
\Output{A partition of the bitmap}
\BlankLine
\emph{special treatment of the first line}\;
\For{$i\leftarrow 2$ \KwTo $l$}{
\emph{special treatment of the first element of line $i$}\;
\For{$j\leftarrow 2$ \KwTo $w$}{\label{forins}
\Left$\leftarrow$ \FindCompress{$Im[i,j-1]$}\;
\Up$\leftarrow$ \FindCompress{$Im[i-1,]$}\;
\This$\leftarrow$ \FindCompress{$Im[i,j]$}\;
\If(\tcp*[h]{O(\Left,\This)==1}){\Left compatible with \This}{\label{lt}
\lIf{\Left $<$ \This}{\Union{\Left,\This}}
\lElse{\Union{\This,\Left}}
}
\If(\tcp*[f]{O(\Up,\This)==1}){\Up compatible with \This}{\label{ut}
\lIf{\Up $<$ \This}{\Union{\Up,\This}}
\tcp{\This is put under \Up to keep tree as flat as possible}\label{cmt}
\lElse{\Union{\This,\Up}}\tcp*[h]{\This linked to \Up}\label{lelse}
}
}
\lForEach{element $e$ of the line $i$}{\FindCompress{p}}
}
\caption{Conjecture Verifier}\label{algo:experiment}
\end{algorithm}\DecMargin{1em}

\begin{lemma}
If there is no perfect matching in $G(A, B)$, then there must be a $k \in \{1, 2, \ldots, m\}$, such that the $k^\textrm{th}$ largest $|P_v(A)|$ across $v \in \mathcal{V}$ and the $k^\textrm{th}$ smallest $|Q_v(B)|$ across $v \in \mathcal{V}$ sum to at most $|\mathcal{C}|$.
\label{lem:reduction_1}
\end{lemma}
\begin{proof}

\end{proof}

\begin{example}
Let $\mathcal{C} = \{A, B, C, D\}$ and $\mathcal{V} = \{1, 2, 3, 4, 5\}$. Consider the following preference profile:
\begin{center}
$D \succ_1 C \succ_1 B \succ_1 A$

$D \succ_2 C \succ_2 B \succ_2 A$

$B \succ_3 A \succ_3 D \succ_3 C$

$B \succ_4 A \succ_4 D \succ_4 C$

$C \succ_5 A \succ_5 D \succ_5 B$
\end{center}
There is no perfect matching in $G(A, B), G(B, C)$ or $G(C, D)$. However, there are perfect matchings in $G(D, A)$ as shown in Figure~\ref{fig:counterexample_relaxation_1}. Despite the existence of perfect matchings, the $3^{\textrm{rd}}$ largest $|P_v(A)|$ is $2$ and the $3^{\textrm{rd}}$ smallest $|Q_v(D)|$ is $2$. Their sum is $4 \leq |\mathcal{C}|$.
\begin{figure}[H]
\centering
\begin{tikzpicture}[scale=0.3]
\node [left] at (0,16) {$P_1(A) = \{A, B, C, D\}$};
\node [left] at (0,12) {$P_2(A) = \{A, B, C, D\}$};
\node [left] at (0,8) {$P_3(A) = \{A, B\}$};
\node [left] at (0,4) {$P_4(A) = \{A, B\}$};
\node [left] at (0,0) {$P_5(A) = \{A, C\}$};
\node [right] at (7,16) {$Q_1(D) = \{A, B, C, D\}$};
\node [right] at (7,12) {$Q_2(D) = \{A, B, C, D\}$};
\node [right] at (7,8) {$Q_3(D) = \{C, D\}$};
\node [right] at (7,4) {$Q_4(D) = \{C, D\}$};
\node [right] at (7,0) {$Q_5(D) = \{B, D\}$};

\draw [ultra thick] (1, 16) to (6, 16);
\draw (1, 16) to (6, 12);
\draw (1, 16) to (6, 8);
\draw (1, 16) to (6, 4);
\draw (1, 16) to (6, 0);
\draw (1, 12) to (6, 16);
\draw (1, 12) to (6, 12);
\draw [ultra thick] (1, 12) to (6, 8);
\draw (1, 12) to (6, 4);
\draw (1, 12) to (6, 0);
\draw (1, 8) to (6, 16);
\draw [ultra thick] (1, 8) to (6, 12);
\draw (1, 8) to (6, 0);
\draw (1, 4) to (6, 16);
\draw (1, 4) to (6, 12);
\draw [ultra thick] (1, 4) to (6, 0);
\draw (1, 0) to (6, 16);
\draw (1, 0) to (6, 12);
\draw (1, 0) to (6, 8);
\draw [ultra thick] (1, 0) to (6, 4);

\draw [fill=white](1,16) circle [radius=1];
\draw [fill=white](1,12) circle [radius=1];
\draw [fill=white](1,8) circle [radius=1];
\draw [fill=white](1,4) circle [radius=1];
\draw [fill=white](1,0) circle [radius=1];

\draw [fill=white](6,16) circle [radius=1];
\draw [fill=white](6,12) circle [radius=1];
\draw [fill=white](6,8) circle [radius=1];
\draw [fill=white](6,4) circle [radius=1];
\draw [fill=white](6,0) circle [radius=1];

\node at (1,16) {$1$};
\node at (1,12) {$2$};
\node at (1,8) {$3$};
\node at (1,4) {$4$};
\node at (1,0) {$5$};

\node at (6,16) {$1$};
\node at (6,12) {$2$};
\node at (6,8) {$3$};
\node at (6,4) {$4$};
\node at (6,0) {$5$};
\end{tikzpicture}
\caption{The Bipartite Graph $G(D, A)$}
\label{fig:counterexample_relaxation_1}
\end{figure}
\label{ex:counterexample_relaxation_1}
\end{example}
